# Supplementary material for: Magnetic coupling to the Advanced Virgo payloads and its impact on the low frequency sensitivity
Source: arXiv:1807.06278 source file (2018-10-23)
Supplement: Supplementary file 1 [file FEA_supplementary_material.pdf]

# Magnetic coupling to the Advanced Virgo payloads and its impact on the low frequency sensitivity

## *Supplementary material*

A. Cirone, A. Chincarini, M. Neri, S. Farinon, G. Gemme, I. Fiori, F. Paoletti, E. Majorana, P. Puppo, P. Rapagnani, P. Ruggi, and B. L. Swinkels

### I. SYSTEM MODELLING: GEOMETRY SIMPLIFICATION AND MODEL MESHING

Building the geometry from sketches can be very difficult, therefore it was imported through the COMSOL CAD Module. Because CAD drawings are made for machining tools, most features and details are a nuisance for FE analysis (Figure S3a).

The first step consists in de-featuring, that is repairing and prune all entities (lines, surfaces and volume domains) that are not correctly recognized as volumes by the Import Module, or that are irrelevant for the simulation. Then we applied two layers of abstraction to the model, both for the sake of mesh simplification (hence simulation time). The first layer deals with critical entities on which a meshing algorithm often does not converge (Figure S3b). These entities include screw holes, bolts, very small features, threadings, etc. The second layer targets mesh simplification at a higher level, trying to reduce the solving time: each volume domain was examined and possibly replaced with the sketched version of itself (Figure S3c). In the end the simplified model was validated against the original drawing.

Meshing the model is a delicate step during which all the elemental volumes are generated. Generally, a balanced and fine mesh leads to better and more stable solutions. Due to the highly irregular geometries, a free mesh made of tetrahedral elements was chosen for the payload (Figure S3d) and the air volume up to the infinite elements, while volumes around the mirror magnets, instead, were meshed with a more refined swept quadrangular elements distribution. The total number of elements in the mesh turned out to be about $7 \cdot 10^5$.

### II. INPUT MIRROR PAYLOAD MEASUREMENT

#### A. Experimental set-up

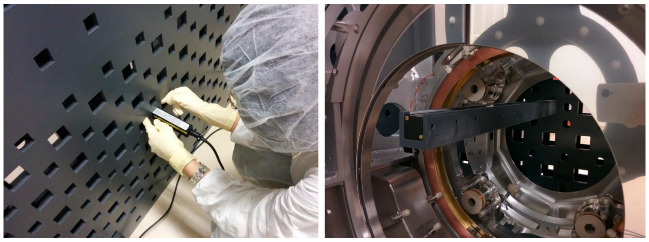

FIG. S1. A focus on the placement of the magnetic probe inside the PVC frame. In addition, a probe-holder rod can make spot measurements along a line inside the volume of the payload.

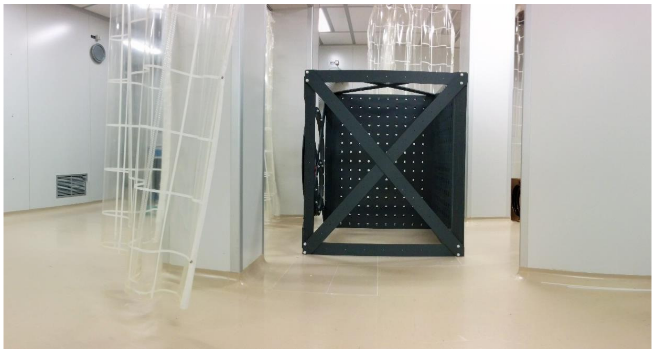

FIG. S2. View of the class 100 clean room and the surrounding site inside which all the experimental apparatus has been set up.

#### B. Validation phase

The validation goal is to identify which electrical configuration best represents the real PAY.

Clearly it is impractical to simulate all the possible 128 configurations for each optimization step. A possible approach would be to simulate only the 7 conditions (the diagonal matrix of the connections) where just one connection is closed and all the others are open. Then, we could find the best approximation to the measurements by linear combination of the diagonal solutions. Unfortunately, the superposition principle does not apply to solutions with eddy currents. In order to solve this issue we resorted to the Design of Experiment (DoE) technique [1, 2] combined with a heuristic algorithm of minimum search.

The DoE approach considers the system under scrutiny as a black box, where only categorical inputs and continuous outputs are measurable. It provides a general rule for dealing with inputs and outputs in order to estimate the system behaviour. We followed the Plackett-Burman implementation [3], which uses, as inputs, the rows of the Hadamard matrix, a square matrix whose entries are only +1 and -1 (or 1 and 0) and whose rows are mutually orthogonal. Such design allows to sample the parameter space reducing the number of tests to perform, but taking into account as many interactions as possible. In addition it approaches the problem without the necessity to define the kind of interaction in the system. That is exactly what we need, since the different electrical configurations of the payload are not independent due to the fact that the current flow changes very much with the connections and the magnetic effect cannot be calculated as a superposition.

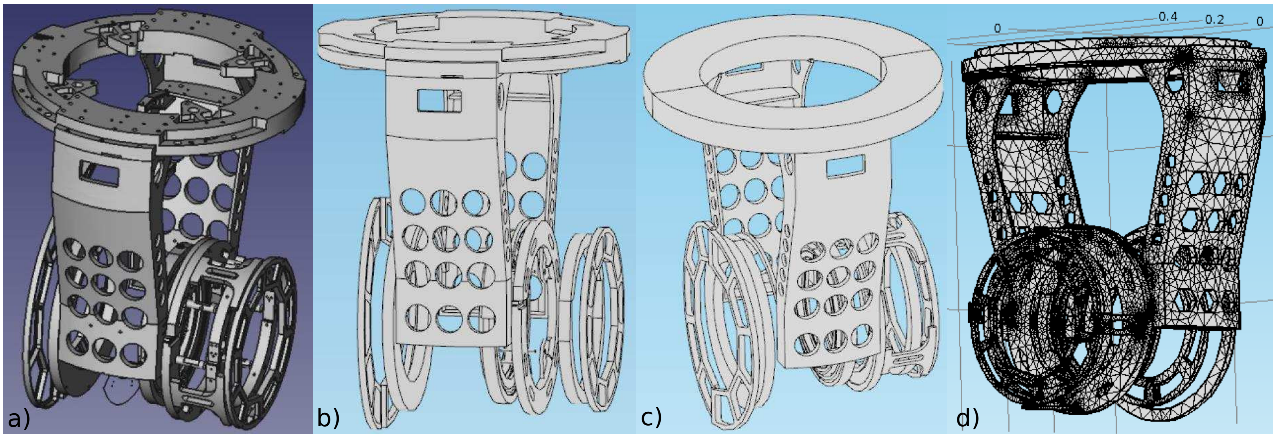


FIG. S3. CAD drawing (a) and finite element models (b-c) of the IMP. The CAD drawing was imported in the FE software and two levels of simplification were applied; d) Meshed payload: the small pieces are meshed finer than the big ones.

In addition, a heuristic optimization procedure was adapted to a discrete parameter space, as each connection can assume only the value 1 or 0. The cost function to be minimized is

$$m_{(k)} = \left| \frac{B^{(k)}_{meas} - B^{(k)}_{sim}}{B^{(k)}_{meas}} \right| \tag{S1}$$

in order to compare the experimental and simulated magnetic field values. We remind that $k$ is the index to the electric connections under test (i.e. possible configurations of the $p = 7$ connections found from the hierarchical analysis). The optimization algorithm is described hereunder:

1. The Hadamard matrix spanning $p$ parameters is used to find $N$ combinations to test
2. A FE simulation is built and solved for each combination
3. The magnetic field obtained from each simulation is compared with the measured one
4. The tested combinations are sorted on the basis of the metric value (Eq. S1)
5. The $n$ parameters ($n < p$) that have the same values in the first two (sorted) combinations are fixed
6. As long as $n \neq 0$, the Hadamard matrix at $p - n$ parameters is used to find new combinations to test

This procedure is iterated until all the parameters are fixed, defining the temporary best configuration. A refinement step looks around the final outcome and allows to check a parameter space subset surrounding the best configuration: all the configurations that differ from the best one by two parameters are tested. This optimization process was first tested with Monte Carlo simulations on complex polynomial functions. These showed that the optimization algorithm finds the global minimum in ≥ 99% of cases. Still, we cannot demonstrate that optimization over the PAY electrical configurations found the global minimum without a exhaustive exploration of the parameter space.

At the end of the optimization procedure we tested 56 configurations out of the possible 128. For each configuration, the cost function in Equation S1 consists of a set of values calculated on the 120 positions were the magnetic probe was placed. All the configurations were sorted according to both the 75th percentile and the median of their distribution. The use of the 75th percentile is a conservative choice to select the configurations whose distribution has a low relative error for the majority of positions. To avoid degeneracy in the configurations, the optimization was carried out using two magnetic field sources ("Big" and "Small" coils). Thus we made less likely that two or more configurations could yield to the same measure results. While the heuristic minimization does not guarantee to reach the global minimum, we are though looking for a solution set whose relative error is below 10%.

## III. EVALUATION OF THE MAGNETS MAGNETIC MOMENT AND POSITIONING ACCURACY

Because of the magnets layout described in Figure 2b of the main text, the total net force on the mirror is null. In practice, neither the total force nor the total torque are null due to non-ideal conditions: *(i)* dis-homogeneity of the **B** field across the mirror area; *(ii)* dis-homogeneity of the magnetic moments; *(iii)* magnets position uncertainty. The last two effects were computed with Monte Carlo computational algorithms, with respect to the payload structure. The first Monte Carlo was used to extract a population of magnetic moments from a normal distribution centred on the nominal value $\mu = 2.20\ mA \times m^2$, with $\sigma_\mu$ being the accuracy provided by the manufacturer (15% of the nominal value), that is $\sigma_\mu = 0.33\ mA \times m^2$. The contribution to the net translational force is:

$$F_z = \nabla B \sum_{i=1}^{4} \mu_i \sim 2(\nabla B)\delta\mu \quad (S2)$$

The second Monte Carlo provided a population of magnet positions, uniformly sampled within a cubic volume of 2 mm per side, centred around the magnet nominal position. This takes into account the gradient spatial distribution. We can similarly write:

$$F_z = \mu \sum_{i=1}^{4} (\frac{\partial B_z}{\partial z})_i (-1)^i = 2\mu\delta(\nabla B) \quad (S3)$$

this time at fixed $\mu$.

## IV. MAGNETIC GRADIENT CALCULATION

The FE model of the payload was placed in a uniform magnetic field $B = 1\,T$ directed along the **x**, **y** and **z** axis alternately. We observed though that the main contribution to the gradient came from $B_z$. We created small volumes ($2 \times 2 \times 2\ mm^3$) around the nominal position of each magnets, which were meshed much finer than the remaining geometry, in order to improve the computation accuracy. The magnetic field gradient was computed in each point of the meshed volume using a finite difference method, for each of the four magnets on the mirror, for each of the 21 equivalent configurations found in the validation step and as a function of frequency. We also took into account the magnets position uncertainty previously evaluated.

## V. FORCE CALCULATION

From Equation 4 of the main text we see that force calculation requires knowledge of both the magnetic gradient and the magnetic moment $\boldsymbol{\mu}$. Three different case studies were considered in the Monte Carlo simulations: one takes into account both the contributions of the magnetic moment tolerance and the position error, while the other two, study the effect of each single uncertainty. The two individual contributions ($\Delta x$ and $\delta\mu$) turns out to be approximately equivalent and hence it is necessary to optimize both of them. We present in Figure S4

the results of the force simulation, based on both the contributions coming from magnetic moment and magnet position uncertainties, as mean values and confidence levels as function of the frequency. We notice that, within the frequency range of interest, from 10 to 100 Hz, the magnetic force level remains almost constant around 2 mN.

Up until now, the force calculation was carried out with a spatially uniform $1\,T$ driving field. The actual force values, instead, depend on the real environmental magnetic field, which will be considered in the magnetic noise estimation.

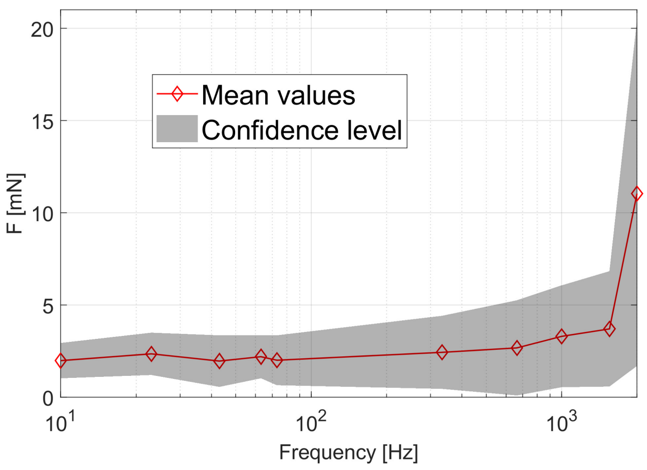


FIG. S4. Monte Carlo simulations of the magnetic force on the mirror, taking into account both magnetic moment and magnet position errors. The diamonds represent the mean values, while the grey band is the associated confidence level.

## REFERENCES

[1] Douglas Montgomery. *Design and Analysis of Experiments*. Hoboken, NJ: John Wiley & Sons, Inc, 8th edition, 2013.
[2] O. Kempthorne. *The Design and Analysis of Experiments*. Wiley eastern private limited, 1952.
[3] R.L. Plackett and J.P. Burman. The design of optimum multifactorial experiments. *Biometrika*, 33, 1946.
